# Supplementary material for: Deploying Image Deblurring across Mobile Devices: A Perspective of Quality and Latency
Source: arXiv:2004.12599 ancillary file (2020-04-27)
Supplement: Supplementary file 1 [file 05-supp_arxiv.pdf]

# Supplementary Material for Deploying Image Deblurring across Mobile Devices: A Perspective of Quality and Latency

Cheng-Ming Chiang\* Yu Tseng Yu-Syuan Xu Hsien-Kai Kuo Yi-Min Tsai  
Guan-Yu Chen Koan-Sin Tan Wei-Ting Wang Yu-Chieh Lin Shou-Yao Roy Tseng  
Wei-Shiang Lin Chia-Lin Yu BY Shen Kloze Kao Chia-Ming Cheng  
Hung-Jen Chen  
MediaTek Inc., Hsinchu, Taiwan

## A. Supplementary

In this supplementary material, we describe detailed network architectures used in the paper for reproducibility in Section A.1. In Section A.2, we provide more visual results of quantization and pruning. Detailed command to evaluate latency on mobile devices are summarized in Section A.3.

### A.1. Network Architecture

In this section, we describe all the network architectures used in the paper in detail. Figure A to Figure F illustrate the architectures listed in Table 2 of our paper. Detailed configuration of each architecture, including kernel size, channel size, stride, and activation, are summarized in Table A to Table F. All the convolutional operations use padding policy, *SAME*, and thus do not state on the table for simplicity. One can refer to these figures and tables to reproduce our experimental results.

For the architecture in Table 3 of the paper, we simply replace *TransposeConv* operation by *DepthToSpace* operation to get UNet-DepthToSpace-Relu and UNet-DepthToSpace-PRelu networks. In UNet-ResizeBilinear-Relu and UNet-ResizeBilinear-PRelu networks, *TransposeConv* is replaced by a *Convolution* operation followed by a *ResizeBilinear* operation. The configuration of the inserted *Convolution* operation has 3 by 3 kernel size and 1 by 1 stride. The number of channel is the same as *TransposeConv*.

### A.2. Visual Quality on Optimized Networks

We provide more visual results of the optimized networks in Figure G to Figure I. It is worth noting that some results of pruned network show slightly better quality than floating-point results. Since the pruning methodology resumes training by using floating-point network as pretrained weight, some minor quality improvement is reasonable.

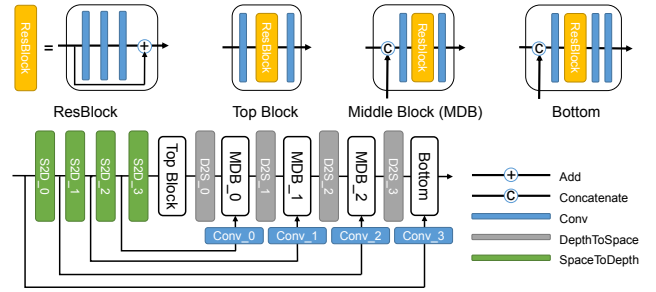

Figure A. SGN\* [2] architecture.

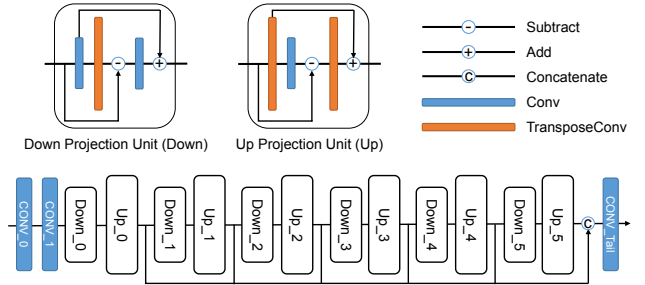

Figure B. DBPN\* [3] architecture.

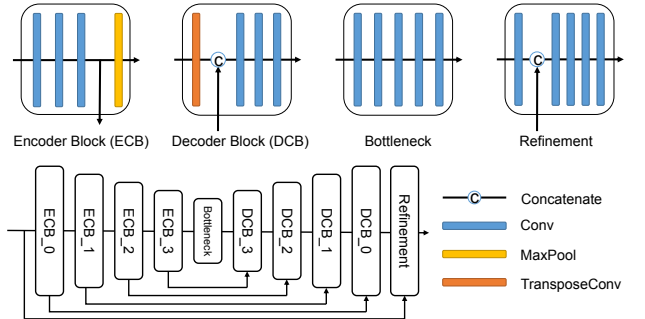

Figure C. U-Net\* [6] architecture.

\*Email: jimmy.chiang@mediatek.com

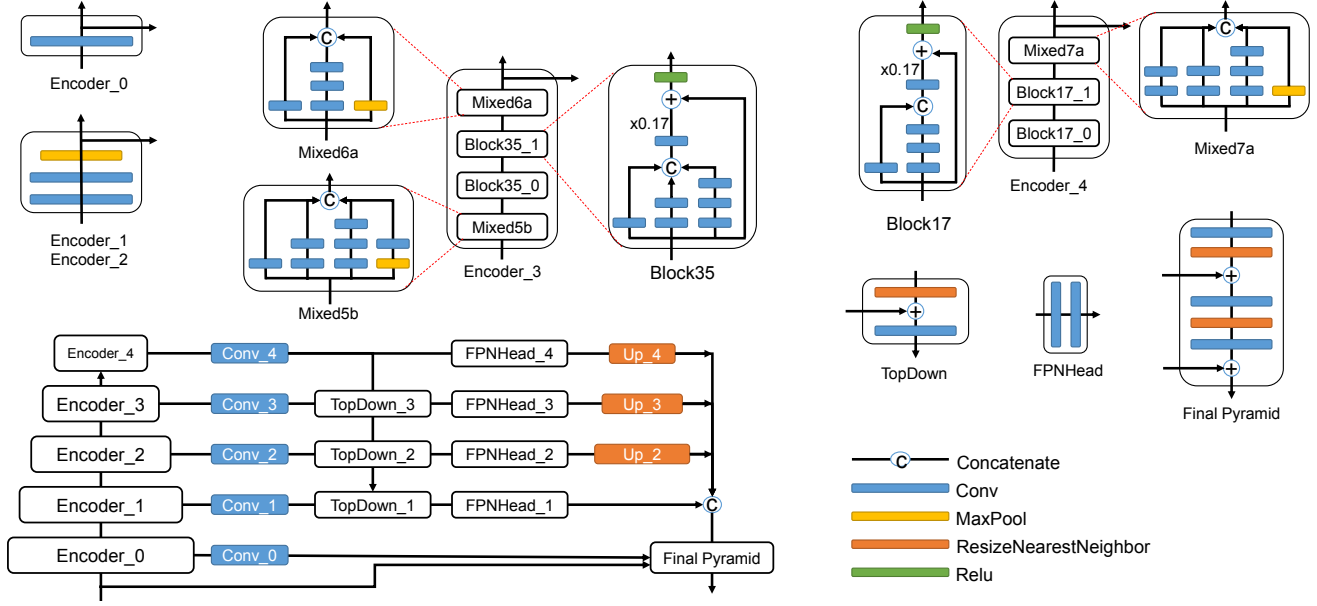

Figure D. Inception-ResNetV2-FPN\* [4] architecture.

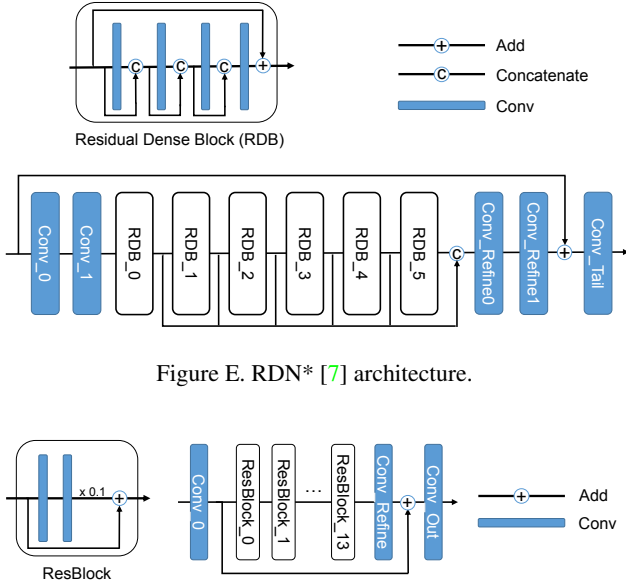

Figure E. RDN\* [7] architecture.

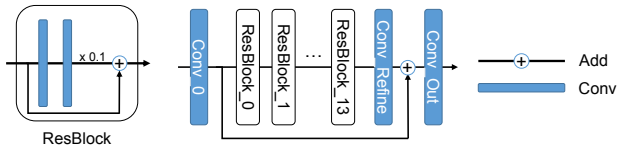

Figure F. EDSR\* [5] architecture.

### A.3. Performance Evaluation

The version of *TFLite Benchmark Tool* [1] used for evaluation is based on the commit of 839dae0. "adb shell taskset f0 /data/local/tmp/benchmark\_model --graph=TFLITE --use\_nnapi=true --allow\_fp16=true --num\_threads=4 --num\_runs=10" is the command used to estimate latency on all the target mobile devices.

For the software version on mobile devices, 10.0.0.205

in Huawei Mate30 Pro 5G, *PDCM00.11.A.12* in OPPO Reno3 5G and *QQ1B.200205.002* in Google Pixel 4.

### References

- [1] TFLite Model Benchmark Tool. <https://github.com/tensorflow/tensorflow/tree/master/tensorflow/lite/tools/benchmark>. 2
- [2] Shuhang Gu, Yawei Li, Luc Van Gool, and Radu Timofte. Self-guided network for fast image denoising. In *Proceedings of the IEEE International Conference on Computer Vision*, pages 2511–2520, 2019. 1
- [3] Muhammad Haris, Gregory Shakhnarovich, and Norimichi Ukita. Deep back-projection networks for super-resolution. In *Proceedings of the IEEE conference on computer vision and pattern recognition*, pages 1664–1673, 2018. 1
- [4] Orest Kupyn, Tetiana Martyniuk, Junru Wu, and Zhangyang Wang. Deblurgan-v2: Deblurring (orders-of-magnitude) faster and better. In *Proceedings of the IEEE International Conference on Computer Vision*, pages 8878–8887, 2019. 2
- [5] Bee Lim, Sanghyun Son, Heewon Kim, Seungjun Nah, and Kyoung Mu Lee. Enhanced deep residual networks for single image super-resolution. In *Proceedings of the IEEE conference on computer vision and pattern recognition workshops*, pages 136–144, 2017. 2
- [6] Olaf Ronneberger, Philipp Fischer, and Thomas Brox. U-net: Convolutional networks for biomedical image segmentation. In *International Conference on Medical image computing and computer-assisted intervention*, pages 234–241. Springer, 2015. 1
- [7] Yulun Zhang, Yapeng Tian, Yu Kong, Bineng Zhong, and Yun Fu. Residual dense network for image super-resolution. In *Proceedings of the IEEE conference on computer vision and pattern recognition*, pages 2472–2481, 2018. 2

Table A. Detailed configuration of U-Net\*.

| Input             | Operator   | Kernel          | Channel              | Stride          | Activation                     |
|-------------------|------------|-----------------|----------------------|-----------------|--------------------------------|
| $720 \times 1280$ | ECB_0      | [3, 3, 3, 2]    | [32, 32, 32, 32]     | [1, 1, 1, 2]    | [Relu, Relu, Relu, Relu]       |
| $360 \times 640$  | ECB_1      | [3, 3, 3, 2]    | [64, 64, 64, 64]     | [1, 1, 1, 2]    | [Relu, Relu, Relu, Relu]       |
| $180 \times 320$  | ECB_2      | [3, 3, 3, 2]    | [128, 128, 128, 128] | [1, 1, 1, 2]    | [Relu, Relu, Relu, Relu]       |
| $90 \times 160$   | ECB_3      | [3, 3, 3, 2]    | [256, 256, 256, 256] | [1, 1, 1, 2]    | [Relu, Relu, Relu, Relu]       |
| $45 \times 80$    | Bottleneck | [3, 3, 3, 3, 3] | [256, 256, 256, 256] | [1, 1, 1, 1]    | [Relu, Relu, Relu, Relu]       |
| $45 \times 80$    | DCB_3      | [4, 3, 3, 3]    | [256, 256, 256, 256] | [2, 1, 1, 1]    | [None, Relu, Relu, Relu]       |
| $90 \times 160$   | DCB_2      | [4, 3, 3, 3]    | [128, 128, 128, 128] | [2, 1, 1, 1]    | [None, Relu, Relu, Relu]       |
| $180 \times 320$  | DCB_1      | [4, 3, 3, 3]    | [64, 64, 64, 64]     | [2, 1, 1, 1]    | [None, Relu, Relu, Relu]       |
| $360 \times 640$  | DCB_0      | [4, 3, 3, 3]    | [32, 32, 32, 32]     | [2, 1, 1, 1]    | [None, Relu, Relu, Relu]       |
| $720 \times 1280$ | Refinement | [3, 3, 3, 1, 1] | [32, 12, 12, 3, 3]   | [1, 1, 1, 1, 1] | [Relu, Relu, Relu, Relu, None] |

Table B. Detailed configuration of EDSR\*.

| Input             | Operator    | Kernel | Channel  | Stride | Activation   |
|-------------------|-------------|--------|----------|--------|--------------|
| $720 \times 1280$ | Conv_0      | 3      | 32       | 1      | Relu         |
| $720 \times 1280$ | ResBlock_1  | [3, 3] | [32, 32] | [1, 1] | [Relu, None] |
| $720 \times 1280$ | ResBlock_2  | [3, 3] | [32, 32] | [1, 1] | [Relu, None] |
| $720 \times 1280$ | ResBlock_3  | [3, 3] | [32, 32] | [1, 1] | [Relu, None] |
| $720 \times 1280$ | ResBlock_4  | [3, 3] | [32, 32] | [1, 1] | [Relu, None] |
| $720 \times 1280$ | ResBlock_5  | [3, 3] | [32, 32] | [1, 1] | [Relu, None] |
| $720 \times 1280$ | ResBlock_6  | [3, 3] | [32, 32] | [1, 1] | [Relu, None] |
| $720 \times 1280$ | ResBlock_7  | [3, 3] | [32, 32] | [1, 1] | [Relu, None] |
| $720 \times 1280$ | ResBlock_8  | [3, 3] | [32, 32] | [1, 1] | [Relu, None] |
| $720 \times 1280$ | ResBlock_9  | [3, 3] | [32, 32] | [1, 1] | [Relu, None] |
| $720 \times 1280$ | ResBlock_10 | [3, 3] | [32, 32] | [1, 1] | [Relu, None] |
| $720 \times 1280$ | ResBlock_11 | [3, 3] | [32, 32] | [1, 1] | [Relu, None] |
| $720 \times 1280$ | ResBlock_12 | [3, 3] | [32, 32] | [1, 1] | [Relu, None] |
| $720 \times 1280$ | ResBlock_13 | [3, 3] | [32, 32] | [1, 1] | [Relu, None] |
| $720 \times 1280$ | Conv_Refine | 3      | 32       | 1      | None         |
| $720 \times 1280$ | Conv_Out    | 3      | 3        | 1      | None         |

Table C. Detailed configuration of RDN\*.

| Input             | Operator     | Kernel       | Channel          | Stride       | Activation               |
|-------------------|--------------|--------------|------------------|--------------|--------------------------|
| $720 \times 1280$ | Conv_0       | 3            | 16               | 1            | None                     |
| $720 \times 1280$ | Conv_1       | 3            | 16               | 1            | None                     |
| $720 \times 1280$ | RDB_0        | [3, 3, 3, 1] | [24, 32, 40, 16] | [1, 1, 1, 1] | [Relu, Relu, Relu, None] |
| $720 \times 1280$ | RDB_1        | [3, 3, 3, 1] | [24, 32, 40, 16] | [1, 1, 1, 1] | [Relu, Relu, Relu, None] |
| $720 \times 1280$ | RDB_2        | [3, 3, 3, 1] | [24, 32, 40, 16] | [1, 1, 1, 1] | [Relu, Relu, Relu, None] |
| $720 \times 1280$ | RDB_3        | [3, 3, 3, 1] | [24, 32, 40, 16] | [1, 1, 1, 1] | [Relu, Relu, Relu, None] |
| $720 \times 1280$ | RDB_4        | [3, 3, 3, 1] | [24, 32, 40, 16] | [1, 1, 1, 1] | [Relu, Relu, Relu, None] |
| $720 \times 1280$ | RDB_5        | [3, 3, 3, 1] | [24, 32, 40, 16] | [1, 1, 1, 1] | [Relu, Relu, Relu, None] |
| $720 \times 1280$ | Conv_Refine0 | 1            | 16               | 1            | None                     |
| $720 \times 1280$ | Conv_Refine1 | 3            | 16               | 1            | None                     |
| $720 \times 1280$ | Conv_Tail    | 3            | 3                | 1            | None                     |

Table D. Detailed configuration of DBPN\*.

| Input             | Operator  | Kernel    | Channel      | Stride    | Activation            |
|-------------------|-----------|-----------|--------------|-----------|-----------------------|
| $720 \times 1280$ | Conv_0    | 3         | 192          | 1         | PRelu                 |
| $720 \times 1280$ | Conv_1    | 3         | 48           | 1         | PRelu                 |
| $720 \times 1280$ | Down_0    | [8, 4, 8] | [48, 48, 48] | [4, 4, 4] | [PRelu, PRelu, PRelu] |
| $180 \times 320$  | Up_0      | [4, 8, 4] | [48, 48, 48] | [4, 4, 4] | [PRelu, PRelu, PRelu] |
| $720 \times 1280$ | Down_1    | [8, 4, 8] | [48, 48, 48] | [4, 4, 4] | [PRelu, PRelu, PRelu] |
| $180 \times 320$  | Up_1      | [4, 8, 4] | [48, 48, 48] | [4, 4, 4] | [PRelu, PRelu, PRelu] |
| $720 \times 1280$ | Down_2    | [8, 4, 8] | [48, 48, 48] | [4, 4, 4] | [PRelu, PRelu, PRelu] |
| $180 \times 320$  | Up_2      | [4, 8, 4] | [48, 48, 48] | [4, 4, 4] | [PRelu, PRelu, PRelu] |
| $720 \times 1280$ | Down_3    | [8, 4, 8] | [48, 48, 48] | [4, 4, 4] | [PRelu, PRelu, PRelu] |
| $180 \times 320$  | Up_3      | [4, 8, 4] | [48, 48, 48] | [4, 4, 4] | [PRelu, PRelu, PRelu] |
| $720 \times 1280$ | Down_4    | [8, 4, 8] | [48, 48, 48] | [4, 4, 4] | [PRelu, PRelu, PRelu] |
| $180 \times 320$  | Up_4      | [4, 8, 4] | [48, 48, 48] | [4, 4, 4] | [PRelu, PRelu, PRelu] |
| $720 \times 1280$ | Down_5    | [8, 4, 8] | [48, 48, 48] | [4, 4, 4] | [PRelu, PRelu, PRelu] |
| $180 \times 320$  | Up_5      | [4, 8, 4] | [48, 48, 48] | [4, 4, 4] | [PRelu, PRelu, PRelu] |
| $720 \times 1280$ | Conv_Tail | 3         | 3            | 1         | None                  |

Table E. Detailed configuration of SGN\*.

| Input             | Operator | Kernel             | Channel                   | Stride             | Activation                           |
|-------------------|----------|--------------------|---------------------------|--------------------|--------------------------------------|
| $720 \times 1280$ | S2D_0    | 2                  | 12                        | –                  | None                                 |
| $360 \times 640$  | S2D_1    | 2                  | 48                        | –                  | None                                 |
| $180 \times 320$  | S2D_2    | 2                  | 192                       | –                  | None                                 |
| $90 \times 160$   | S2D_3    | 2                  | 768                       | –                  | None                                 |
| $45 \times 80$    | TopBlock | [3, 3, 3, 3, 3]    | [512, 512, 512, 512, 512] | [1, 1, 1, 1, 1]    | [Relu, Relu, Relu, None, Relu]       |
| $45 \times 80$    | D2S_0    | 2                  | 128                       | –                  | None                                 |
| $90 \times 160$   | Conv_0   | 3                  | 256                       | 1                  | Relu                                 |
| $90 \times 160$   | MDB_0    | [3, 3, 3, 3, 3]    | [256, 256, 256, 256, 256] | [1, 1, 1, 1, 1]    | [Relu, Relu, Relu, None, Relu]       |
| $90 \times 160$   | D2S_1    | 2                  | 64                        | –                  | None                                 |
| $180 \times 320$  | Conv_1   | 3                  | 128                       | 1                  | Relu                                 |
| $180 \times 320$  | MDB_1    | [3, 3, 3, 3, 3]    | [128, 128, 128, 128, 128] | [1, 1, 1, 1, 1]    | [Relu, Relu, Relu, None, Relu]       |
| $180 \times 320$  | D2S_2    | 2                  | 32                        | –                  | None                                 |
| $360 \times 640$  | Conv_2   | 3                  | 64                        | 1                  | Relu                                 |
| $360 \times 640$  | MDB_2    | [3, 3, 3, 3, 3]    | [64, 64, 64, 64, 64]      | [1, 1, 1, 1, 1]    | [Relu, Relu, Relu, None, Relu]       |
| $360 \times 640$  | D2S_3    | 2                  | 16                        | –                  | None                                 |
| $720 \times 1280$ | Conv_3   | 3                  | 32                        | 1                  | Relu                                 |
| $720 \times 1280$ | Bottom   | [3, 3, 3, 3, 3, 3] | [32, 32, 32, 32, 32, 3]   | [1, 1, 1, 1, 1, 1] | [Relu, Relu, Relu, None, Relu, None] |

Kernel in D2S and S2D operations represent block\_size.

Table F. Detailed configuration of Inception-ResNetV2-FPN\*.

| Input             | Operator            | Kernel          | Channel                                                                | Stride          | Activation                     |
|-------------------|---------------------|-----------------|------------------------------------------------------------------------|-----------------|--------------------------------|
| $720 \times 1280$ | Encoder_0           | 3               | 128                                                                    | 2               | Relu                           |
| $360 \times 640$  | Encoder_1           | [3, 3, 3]       | [128, 128, 128]                                                        | [1, 1, 2]       | [Relu, Relu, None]             |
| $179 \times 319$  | Encoder_2           | [1, 3, 3]       | [128, 128, 128]                                                        | [1, 1, 2]       | [Relu, Relu, None]             |
| $89 \times 159$   | Mixed5b-branch0     | 1               | 96                                                                     | 1               | Relu                           |
| $89 \times 159$   | Mixed5b-branch1     | [1, 5]          | [48, 64]                                                               | [1, 1]          | [Relu, Relu]                   |
| $89 \times 159$   | Mixed5b-branch2     | [1, 3, 3]       | [64, 96, 96]                                                           | [1, 1, 1]       | [Relu, Relu, Relu]             |
| $89 \times 159$   | Mixed5b-branch3     | [3, 1]          | [128, 64]                                                              | [1, 1]          | [None, Relu]                   |
| $89 \times 159$   | Block35_0-branch0   | 1               | 32                                                                     | 1               | Relu                           |
| $89 \times 159$   | Block35_0-branch1   | [1, 3]          | [32, 32]                                                               | [1, 1]          | [Relu, Relu]                   |
| $89 \times 159$   | Block35_0-branch2   | [1, 3, 3]       | [32, 48, 64]                                                           | [1, 1, 1]       | [Relu, Relu, Relu]             |
| $89 \times 159$   | Block35_0-finalconv | 1               | 320                                                                    | 1               | Relu                           |
| $89 \times 159$   | Block35_1-branch0   | 1               | 32                                                                     | 1               | Relu                           |
| $89 \times 159$   | Block35_1-branch1   | [1, 3]          | [32, 32]                                                               | [1, 1]          | [Relu, Relu]                   |
| $89 \times 159$   | Block35_1-branch2   | [1, 3, 3]       | [32, 48, 64]                                                           | [1, 1, 1]       | [Relu, Relu, Relu]             |
| $89 \times 159$   | Block35_1-finalconv | 1               | 320                                                                    | 1               | Relu                           |
| $89 \times 159$   | Mixed6a-branch0     | 3               | 256                                                                    | 2               | Relu                           |
| $89 \times 159$   | Mixed6a-branch1     | [1, 3, 3]       | [256, 256, 256]                                                        | [1, 1, 2]       | [Relu, Relu, Relu]             |
| $89 \times 159$   | Mixed6a-branch2     | 3               | 320                                                                    | 2               | None                           |
| $45 \times 80$    | Block17_0-branch0   | 1               | 192                                                                    | 1               | Relu                           |
| $45 \times 80$    | Block17_0-branch1   | [1, 1x7, 7x1]   | [128, 160, 192]                                                        | [1, 1, 1]       | [Relu, Relu, Relu]             |
| $45 \times 80$    | Block17_0-finalconv | 1               | 832                                                                    | 1               | Relu                           |
| $45 \times 80$    | Block17_1-branch0   | 1               | 192                                                                    | 1               | Relu                           |
| $45 \times 80$    | Block17_1-branch1   | [1, 1x7, 7x1]   | [128, 160, 192]                                                        | [1, 1, 1]       | [Relu, Relu, Relu]             |
| $45 \times 80$    | Block17_1-finalconv | 1               | 832                                                                    | 1               | Relu                           |
| $45 \times 80$    | Mixed7a-branch0     | [1, 3]          | [256, 256]                                                             | [1, 2]          | [Relu, Relu]                   |
| $45 \times 80$    | Mixed7a-branch1     | [1, 3]          | [256, 256]                                                             | [1, 2]          | [Relu, Relu]                   |
| $45 \times 80$    | Mixed7a-branch2     | [1, 3, 3]       | [256, 256, 256]                                                        | [1, 1, 2]       | [Relu, Relu, Relu]             |
| $45 \times 80$    | Mixed7a-branch3     | 3               | 832                                                                    | 2               | None                           |
| $23 \times 40$    | Conv_4              | 1               | 256                                                                    | 1               | None                           |
| $45 \times 80$    | Conv_3              | 1               | 256                                                                    | 1               | None                           |
| $89 \times 159$   | Conv_2              | 1               | 256                                                                    | 1               | None                           |
| $179 \times 319$  | Conv_1              | 1               | 256                                                                    | 1               | None                           |
| $360 \times 640$  | Conv_0              | 1               | 128                                                                    | 1               | None                           |
| $23 \times 40$    | TopDown_3           | [-, 3]          | $[45 \times 80 \times 256, 256]^1$                                     | [-, 1]          | [None, Relu]                   |
| $45 \times 80$    | TopDown_2           | [-, 3]          | $[89 \times 159 \times 256, 256]^1$                                    | [-, 1]          | [None, Relu]                   |
| $89 \times 159$   | TopDown_1           | [-, 3]          | $[179 \times 319 \times 256, 256]^1$                                   | [-, 1]          | [None, Relu]                   |
| $23 \times 40$    | FPNHead_4           | [3, 3]          | [128, 128]                                                             | [1, 1]          | [Relu, Relu]                   |
| $45 \times 80$    | FPNHead_3           | [3, 3]          | [128, 128]                                                             | [1, 1]          | [Relu, Relu]                   |
| $89 \times 159$   | FPNHead_2           | [3, 3]          | [128, 128]                                                             | [1, 1]          | [Relu, Relu]                   |
| $179 \times 319$  | FPNHead_1           | [3, 3]          | [128, 128]                                                             | [1, 1]          | [Relu, Relu]                   |
| $23 \times 40$    | Up_4                | -               | $179 \times 319 \times 128$                                            | 1               | None                           |
| $45 \times 80$    | Up_3                | -               | $179 \times 319 \times 128$                                            | 1               | None                           |
| $89 \times 159$   | Up_2                | -               | $179 \times 319 \times 128$                                            | 1               | None                           |
| $179 \times 319$  | FinalPyramid        | [3, -, 3, -, 3] | $[128, 360 \times 640 \times 128, 64, 720 \times 1280 \times 64, 3]^2$ | [1, -, 1, -, 1] | [Relu, None, Relu, None, Tanh] |

<sup>1</sup> The first operation in TopDown module is RESIZE\_NEAREST\_NEIGHBOR. The configuration listed in Channel represents output\_height  $\times$  output\_width  $\times$  output\_channel.

<sup>2</sup> The second and fourth operation in FinalPyramid module is RESIZE\_NEAREST\_NEIGHBOR. The configuration listed in Channel represents output\_height  $\times$  output\_width  $\times$  output\_channel.

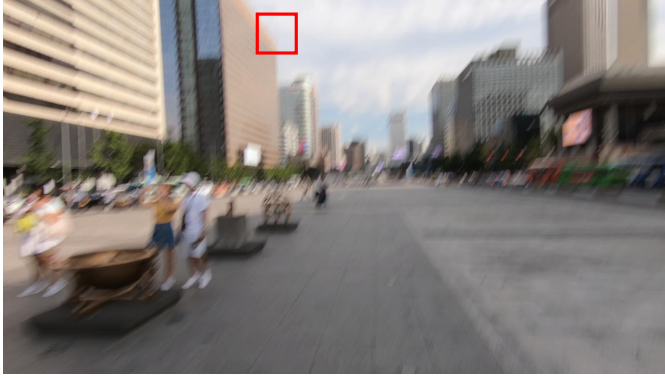

(a) Input Image

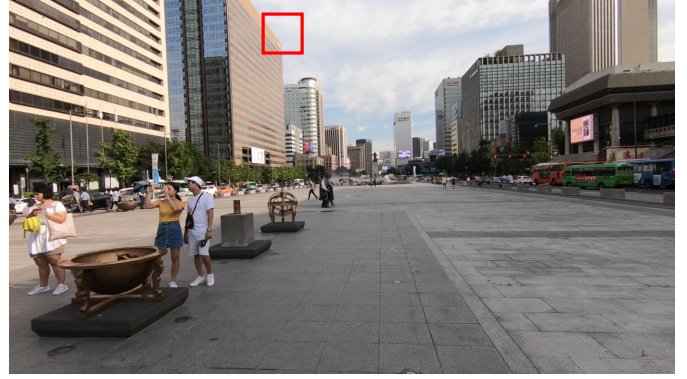

(b) Ground Truth Image

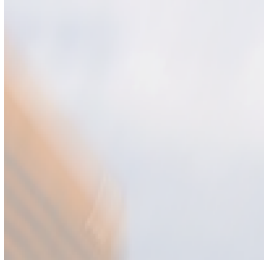

(c) Input Patch

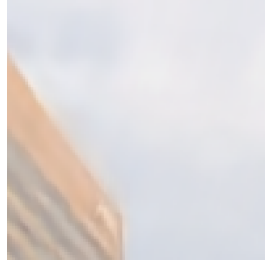

(d) Floating-point

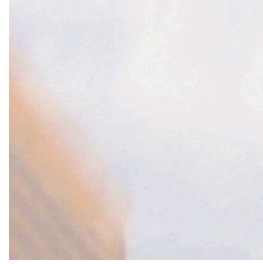

(e) 8-bit PTQ

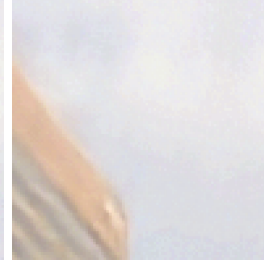

(f) 8-bit QAT

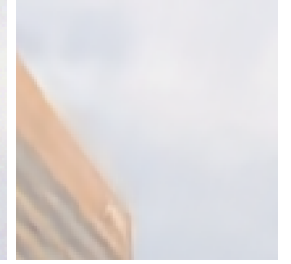

(g) 16-bit PTQ

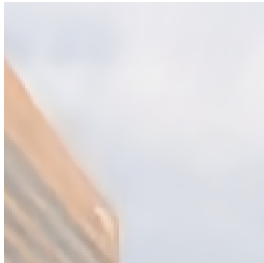

(h) -5% MAC

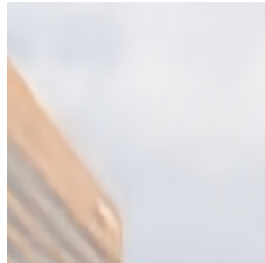

(i) -10% MAC

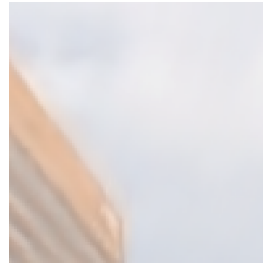

(j) -30% MAC

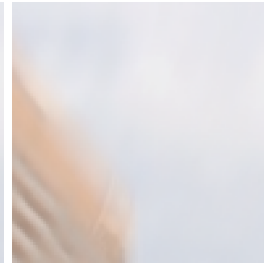

(k) -50% MAC

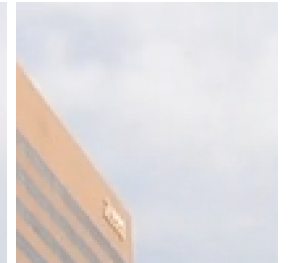

(l) Ground Truth Patch

Figure G. Visual results of UNet-ResizeBilinear-PReLU with network quantization and pruning. (e)(f)(g) represent different quantization settings as in Table 4. (h)(i)(j)(k) show the results of pruning given different MAC reduction targets. The image is selected from *001/00000029.png* in REDS validation set.

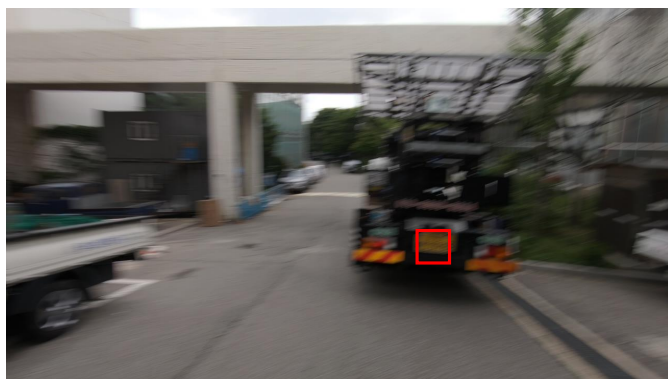

(a) Input Image

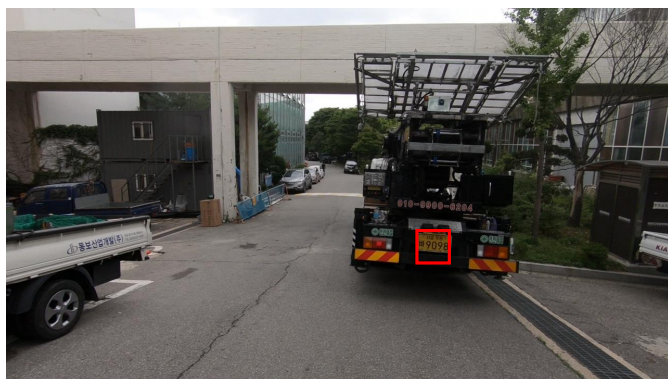

(b) Ground Truth Image

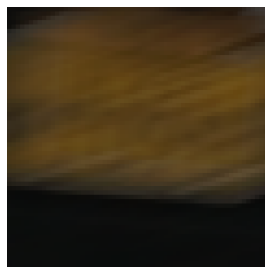

(c) Input Patch

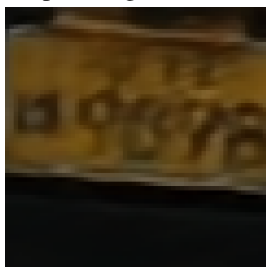

(d) Floating-point

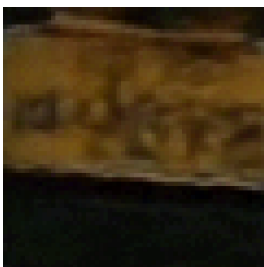

(e) 8-bit PTQ

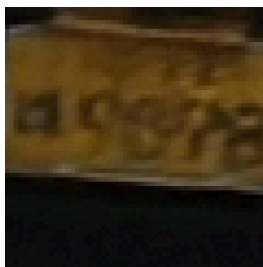

(f) 8-bit QAT

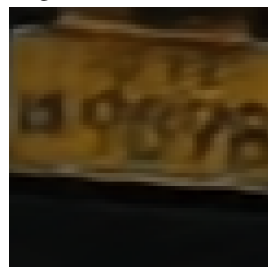

(g) 16-bit PTQ

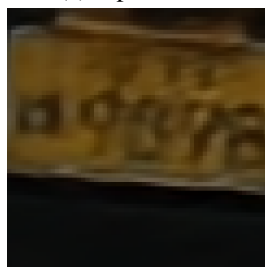

(h) -5% MAC

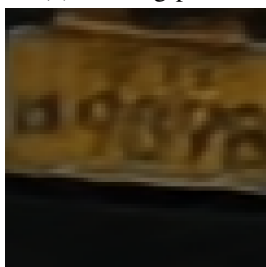

(i) -10% MAC

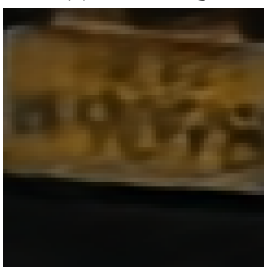

(j) -30% MAC

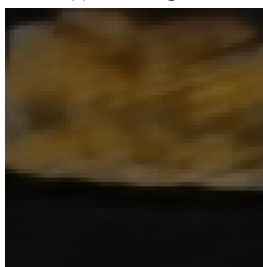

(k) -50% MAC

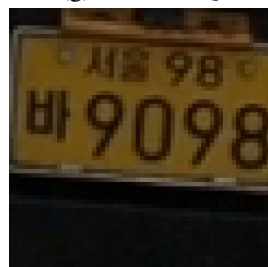

(l) Ground Truth Patch

Figure H. Visual results of UNet-ResizeBilinear-PReLU with network quantization and pruning. (e)(f)(g) represent different quantization settings as in Table 4. (h)(i)(j)(k) show the results of pruning given different MAC reduction targets. The image is selected from 005/00000069.png in REDS validation set.

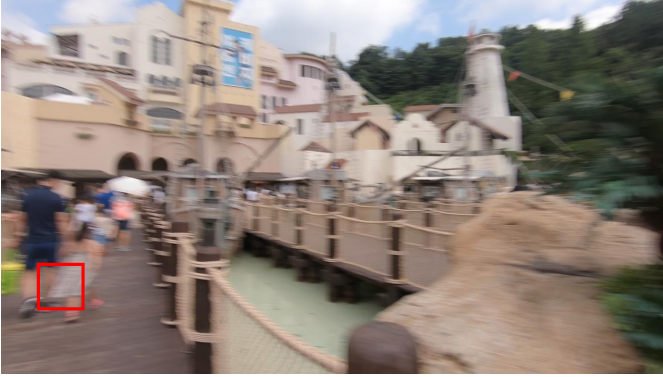

(a) Input Image

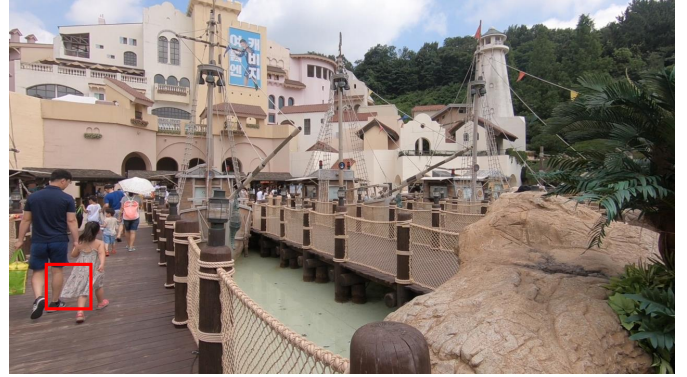

(b) Ground Truth Image

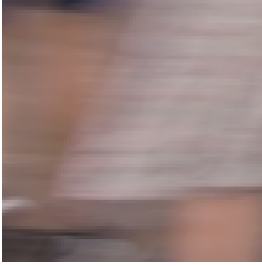

(c) Input Patch

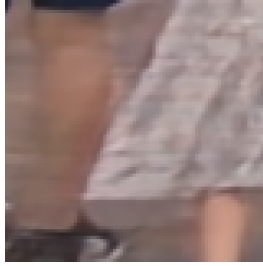

(d) Floating-point

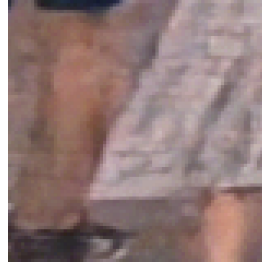

(e) 8-bit PTQ

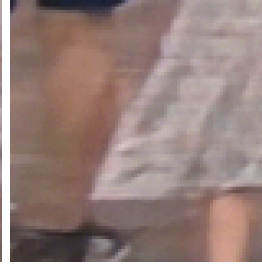

(f) 8-bit QAT

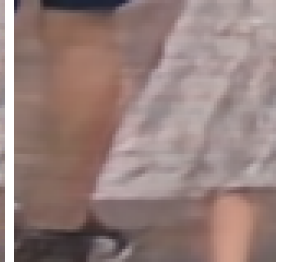

(g) 16-bit PTQ

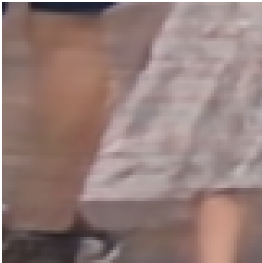

(h) -5% MAC

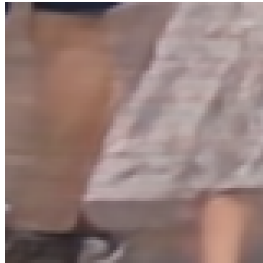

(i) -10% MAC

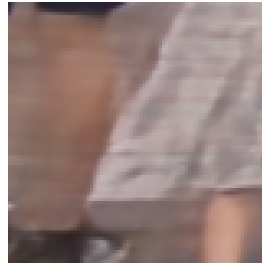

(j) -30% MAC

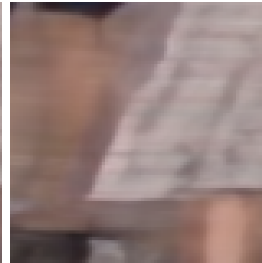

(k) -50% MAC

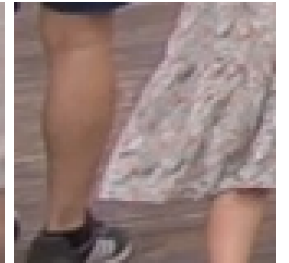

(l) Ground Truth Patch

Figure I. Visual results of UNet-ResizeBilinear-PRelu with network quantization and pruning. (e)(f)(g) represent different quantization settings as in Table 4. (h)(i)(j)(k) show the results of pruning given different MAC reduction targets. The image is selected from 006/00000089.png in REDS validation set.
